# Supplementary material for: Teaching a Formalized Logical Calculus
Source: arXiv:2002.12555 source file (2020-02-28)
Supplement: Supplementary file 1 [file Appendix.pdf]

```
datatype 'a "term" =  
  Var nat |  
  Fun 'a <'a term list>
```

```
datatype ('a, 'b) form =  
  FF ("⊥") |  
  TT ("⊤") |  
  Pre 'b <'a term list> |  
  Con <('a, 'b) form> <('a, 'b) form> |  
  Dis <('a, 'b) form> <('a, 'b) form> |  
  Imp <('a, 'b) form> <('a, 'b) form> |  
  Neg <('a, 'b) form> |  
  Uni <('a, 'b) form> |  
  Exi <('a, 'b) form>
```

```
datatype 'a hterm = HFun 'a <'a hterm list>
```

**definition** shift **where**

```
<shift e v z  $\equiv$   $\lambda n$ . if n < v then e n else if n = v then z else e (n - 1)>
```

**fun** semantics\_term **and** semantics\_list **where**

```
<semantics_term e f (Var n) = e n> |
```

```
<semantics_term e f (Fun i l) = f i (semantics_list e f l)> |
```

```
<semantics_list e f [] = []> |
```

```
<semantics_list e f (t # l) = semantics_term e f t # semantics_list e f l>
```

**fun** semantics **where**

```
<semantics e f g  $\perp$  = False> |
```

```
<semantics e f g  $\top$  = True> |
```

```
<semantics e f g (Pre i l) = g i (semantics_list e f l)> |
```

```
<semantics e f g (Con p q) = (semantics e f g p  $\wedge$  semantics e f g q)> |
```

```
<semantics e f g (Dis p q) = (semantics e f g p  $\vee$  semantics e f g q)> |
```

```
<semantics e f g (Imp p q) = (semantics e f g p  $\longrightarrow$  semantics e f g q)> |
```

```
<semantics e f g (Neg p) = ( $\neg$  semantics e f g p)> |
```

```
<semantics e f g (Uni p) = ( $\forall z$ . semantics (shift e 0 z) f g p)> |
```

```
<semantics e f g (Exi p) = ( $\exists z$ . semantics (shift e 0 z) f g p)>
```

```
fun new_term and new_list where
  <new_term c (Var n) = True> |
  <new_term c (Fun i l) = (if i = c then False else new_list c l)> |
  <new_list c [] = True> |
  <new_list c (t # l) = (if new_term c t then new_list c l else False)>
```

```
fun new where
  <new c  $\perp$  = True> |
  <new c  $\top$  = True> |
  <new c (Pre i l) = new_list c l> |
  <new c (Con p q) = (if new c p then new c q else False)> |
  <new c (Dis p q) = (if new c p then new c q else False)> |
  <new c (Imp p q) = (if new c p then new c q else False)> |
  <new c (Neg p) = new c p> |
  <new c (Uni p) = new c p> |
  <new c (Exi p) = new c p>
```

```
fun news where
  <news c [] = True> |
  <news c (p # x) = (if new c p then news c x else False)>
```

**fun** inc\_term **and** inc\_list **where**

```
<inc_term (Var n) = Var (n + 1)> |  
<inc_term (Fun i l) = Fun i (inc_list l)> |  
<inc_list [] = []> |  
<inc_list (t # l) = inc_term t # inc_list l>
```

**fun** sub\_term **and** sub\_list **where**

```
<sub_term v s (Var n) = (if n < v then Var n else if n = v then s else Var (n - 1))> |  
<sub_term v s (Fun i l) = Fun i (sub_list v s l)> |  
<sub_list v s [] = []> |  
<sub_list v s (t # l) = sub_term v s t # sub_list v s l>
```

**fun** sub **where**

```
<sub v s  $\perp$  =  $\perp$ > |  
<sub v s  $\top$  =  $\top$ > |  
<sub v s (Pre i l) = Pre i (sub_list v s l)> |  
<sub v s (Con p q) = Con (sub v s p) (sub v s q)> |  
<sub v s (Dis p q) = Dis (sub v s p) (sub v s q)> |  
<sub v s (Imp p q) = Imp (sub v s p) (sub v s q)> |  
<sub v s (Neg p) = Neg (sub v s p)> |  
<sub v s (Uni p) = Uni (sub (v + 1) (inc_term s) p)> |  
<sub v s (Exi p) = Exi (sub (v + 1) (inc_term s) p)>
```

```
fun member where
  <member p [] = False> |
  <member p (q # x) = (if p = q then True else member p x)>
```

```
fun ext where
  <ext y [] = True> |
  <ext y (p # x) = (if member p y then ext y x else False)>
```

```

inductive sequent_calculus ("⊢_" 0) where
  <⊢ Pre i l # Neg (Pre i l) # x> |
  <⊢ Neg ⊥ # x> |
  <⊢ ⊤ # x> |
  <⊢ p # x ⇒ ⊢ Neg (Neg p) # x> |
  <⊢ Neg p # Neg q # x ⇒ ⊢ Neg (Con p q) # x> |
  <⊢ p # q # x ⇒ ⊢ Dis p q # x> |
  <⊢ Neg p # q # x ⇒ ⊢ Imp p q # x> |
  <⊢ p # x ⇒ ⊢ q # x ⇒ ⊢ Con p q # x> |
  <⊢ Neg p # x ⇒ ⊢ Neg q # x ⇒ ⊢ Neg (Dis p q) # x> |
  <⊢ p # x ⇒ ⊢ Neg q # x ⇒ ⊢ Neg (Imp p q) # x> |
  <⊢ sub 0 t p # x ⇒ ⊢ Exi p # x> |
  <⊢ Neg (sub 0 t p) # x ⇒ ⊢ Neg (Uni p) # x> |
  <⊢ sub 0 (Fun i []) p # x ⇒ news i (p # x) ⇒ ⊢ Uni p # x> |
  <⊢ Neg (sub 0 (Fun i []) p) # x ⇒ news i (p # x) ⇒ ⊢ Neg (Exi p) # x> |
  <⊢ x ⇒ ext y x ⇒ ⊢ y>

```

**abbreviation** herbrand\_valid (">> \_" 0) **where**

$\langle (>> p :: (\text{nat}, \text{nat}) \text{ form}) \equiv \forall (e :: \_ \Rightarrow \text{nat hterm}) f g. \text{ semantics } e f g p \rangle$

**theorem** complete\_sound:  $\langle >> p \Rightarrow \Vdash [p] \rangle \langle \Vdash [q] \Rightarrow \text{ semantics } e f g q \rangle$

**corollary**  $\langle \langle \gg p \rangle \longleftrightarrow (\Vdash [p]) \rangle$
